# Supplementary material for: Object-Aware Query Perturbation for Cross-Modal Image-Text Retrieval
Source: arXiv:2407.12346 source file (2024-09-25)
Supplement: Supplementary file 1 [file eccv_supp_tab1.tex]

\begin{table}
    \centering
\caption{Caption}
\label{tab:my_label}
    \begin{tabular}{lrrrrrrrrrrr}
    \toprule
         &  \textasciitilde 10\%&  \textasciitilde 20\%&  \textasciitilde 30\%&  \textasciitilde 40\%&  \textasciitilde 50\%&  \textasciitilde 60\%&  \textasciitilde 70\%&  \textasciitilde 80\%& \textasciitilde 90\% &\textasciitilde 100\% &mR@1\\
    \midrule
         &  \multicolumn{11}{c}{Flickr-30K T2I}\\
    \midrule
         BLIP2&  81.33 &  85.00 &  90.11 &  87.59 &  88.92 &  91.29 &  90.89 &  90.67 &  92.56 & 90.38 
&88.75 
\\
         ~~w/Q-Pert.(E)&  84.00 &  85.00 &  90.97 &  87.41 &  89.19 &  91.00 &  90.89 &  90.67 &  92.56 & 90.13 
&89.10 
\\
         ~~w/Q-Pert.(D)&  84.00 &  85.67 &  90.11 &  87.59 &  89.32 &  91.29 &  90.36 &  90.44 &  92.31 & 90.77 
&89.11 
\\
    \midrule
         &  \multicolumn{11}{c}{Flickr-30K I2T}\\
    \midrule
         BLIP2
&  93.33 &  98.33 &  97.85 &  96.30 &  99.32 &  96.43 &  96.43 &  97.78 &  98.72 & 98.08 
&97.23 
\\
 ~~w/Q-Pert.(E)
& 93.33 & 98.33 & 97.85 & 98.15 & 99.32 & 97.14 & 96.43 & 97.78 & 98.72 & 98.72 
&97.55 
\\
 ~~w/Q-Pert.(D)& 93.33 & 98.33 & 96.77 & 97.22 & 99.32 & 97.14 & 96.43 & 97.78 & 98.72 & 98.08 
&97.29 

\\
    \midrule
        & \multicolumn{11}{c}{COCO-5K T2I}\\
    \midrule
 BLIP2
& 59.87 & 64.37 & 66.66 & 72.11 & 75.01 & 72.16 & 75.93 & 75.45 & 76.26 & 77.94 
&71.09 
\\
 ~~w/Q-Pert.(E)
& 60.17 & 64.39 & 66.66 & 72.11 & 75.20 & 72.16 & 75.84 & 75.35 & 76.26 & 78.00 
&71.14 
\\
 ~~w/Q-Pert.(D)& 60.09 & 64.39 & 67.03 & 71.96 & 75.48 & 71.98 & 75.93 & 75.25 & 76.40 & 77.73 
&71.15 
\\
    \midrule
        & \multicolumn{11}{c}{COCO-5K I2T}\\
    \midrule
 BLIP2
& 80.18 & 82.50 & 81.61 & 88.24 & 90.70 & 87.65 & 91.59 & 92.57 & 89.93 & 91.51 
&87.43 
\\
~~w/Q-Pert.(E)
& 80.93 & 82.39 & 82.23 & 88.05 & 90.70 & 87.35 & 92.04 & 92.08 & 89.93 & 91.51 
&87.52 
\\
 ~~w/Q-Pert.(D)& 79.85 & 82.73 & 82.38 & 88.24 & 90.70 & 87.35 & 92.48 & 92.57 & 91.37 & 91.51 
&87.69 
\\
    \midrule
        & \multicolumn{11}{c}{Flickr-FG T2I}\\
    \midrule
BLIP2&  85.33 &  90.00 &  92.69 &  90.93 &  92.16 &  93.43 &  93.04 &  93.11 &  95.64 & 92.31 
&91.79 
\\
         ~~w/Q-Pert.(E)&  86.67 &  90.67 &  92.90 &  91.11 &  92.57 &  93.00 &  92.86 &  92.44 &  95.38 & 92.69 
&91.98 
\\
         ~~w/Q-Pert.(D)&  86.67 &  90.67 &  92.47 &  91.30 &  92.30 &  93.43 &  92.86 &  93.11 &  95.38 & 92.95 
&92.06 
\\
    \midrule
         &  \multicolumn{11}{c}{Flickr-FG I2T}\\
    \midrule
         BLIP2
&  100.00 &  100.00 &  98.92 &  99.07 &  99.32 &  97.86 &  98.21 &  96.67 &  100.00 & 97.44 
&98.50 
\\
 ~~w/Q-Pert.(E)
& 100.00 & 100.00 & 98.92 & 98.15 & 99.32 & 97.86 & 98.21 & 98.89 & 100.00 & 97.44 
&98.60 
\\
 ~~w/Q-Pert.(D)& 100.00 & 100.00 & 98.92 & 99.07 & 99.32 & 97.86 & 98.21 & 97.78 & 100.00 & 97.44 
&98.60 
\\
    \midrule
        & \multicolumn{11}{c}{COCO-FG T2I}\\
    \midrule
 BLIP2
& 63.93 & 68.25 & 71.65 & 77.43 & 79.12 & 77.96 & 81.33 & 79.80 & 81.58 & 80.85 
&75.71 
\\
 ~~w/Q-Pert.(E)
& 64.00 & 68.39 & 71.59 & 77.46 & 79.35 & 77.96 & 81.06 & 80.30 & 81.58 & 80.80 
&75.77 
\\
 ~~w/Q-Pert.(D)& 64.06 & 68.41 & 71.65 & 77.46 & 79.21 & 78.02 & 81.24 & 80.30 & 81.29 & 80.95 
&75.78 
\\
    \midrule
        & \multicolumn{11}{c}{COCO-FG I2T}\\
    \midrule
 BLIP2
& 81.18 & 84.94 & 85.94 & 90.07 & 92.79 & 92.90 & 92.04 & 94.06 & 92.09 & 94.43 
&89.83 
\\
~~w/Q-Pert.(E)
& 81.93 & 85.17 & 85.94 & 90.26 & 92.79 & 93.21 & 91.59 & 93.56 & 92.81 & 94.43 
&89.98 
\\
 ~~w/Q-Pert.(D)& 81.27 & 84.70 & 86.24 & 90.26 & 93.95 & 92.28 & 92.04 & 93.56 & 92.09 & 94.43 
&89.87 
\\
\bottomrule
    \end{tabular}

\end{table}
