# Supplementary material for: Object-Aware Query Perturbation for Cross-Modal Image-Text Retrieval
Source: arXiv:2407.12346 source file (2024-09-25)
Supplement: Supplementary file 2 [file eccv_supp_tab2.tex]

\begin{table}
\caption{Hoge}
    \begin{minipage}[c]{.5\hsize}
        \centering
        
        \begin{tabular}{llrrrrr}
        \toprule
            && \multicolumn{5}{c}{scale}\\
        \midrule
            &&  2 &  4&  6&  8& 10\\
        \midrule
            &$\bar{S}$ &  81.33&  82.67&  81.33&  80& 81.33
\\
            &1-$\bar{S}$ &  82.67&  82.67&  80&  81.33& 84
\\
            &$\bar{S}$-0.5 &  81.33&  81.33&  81.33&  82.67& 82.67
\\
            &0.5-$\bar{S}$&  81.33&  82.67&  81.33&  81.33& 81.33
\\
            &constant&  82.67&  81.33&  81.33&  81.33& 84
\\
        \bottomrule
        \end{tabular}
        \subcaption{R@1 small(10\%)}
    \end{minipage}
    \begin{minipage}[c]{.5\hsize}
        \centering
        \begin{tabular}{llrrrrr}
        \toprule
            && \multicolumn{5}{c}{scale}\\
        \midrule
            &&  2 &  4&  6&  8& 10\\
        \midrule
            &$\bar{S}$ &  88.73&  88.65&  88.67&  88.67& 88.77
\\
            &1-$\bar{S}$ &  88.85&  88.63&  88.63&  88.93& 88.62
\\
            &$\bar{S}$-0.5 &  88.69&  88.41&  88.75&  88.46& 88.52
\\
            &0.5-$\bar{S}$&  88.53&  88.8&  88.81&  88.72& 88.63
\\
            &constant&  88.63&  88.95&  88.93&  88.67& 88.76
\\
        \bottomrule
        \end{tabular}
        \subcaption{R@1}
    \end{minipage}
    \label{tab:scale_sensitivity}
\end{table}

\begin{table}
    \caption{Hoge}
    \begin{minipage}[c]{.5\hsize}
        \centering
        \begin{tabular}{llrrrrr}
        \toprule
            && \multicolumn{5}{c}{Contribution ratio
}\\
        \midrule
            &&  0.80&  0.85&  0.90&  0.95& 0.99
\\
        \midrule
            &$\bar{S}$ &  81.33&  81.33&  81.33&  81.33& 
82.67
\\
            &1-$\bar{S}$ &  81.33&  84&  84&  82.67& 
81.33
\\
            &$\bar{S}$-0.5 &  81.33&  80&  80&  80& 
81.33
\\
            &0.5-$\bar{S}$&  81.33&  81.33&  80&  81.33& 
81.33
\\
            &constant&  81.33&  81.33&  85.33&  82.67& 84
\\
        \bottomrule
        \end{tabular}
        \subcaption{R@1 small(10\%)}
    \end{minipage}
    \begin{minipage}[c]{.5\hsize}
        \centering
        \begin{tabular}{llrrrrr}
        \toprule
            && \multicolumn{5}{c}{Contribution ratio
}\\
        \midrule
            &&  0.80&  0.85&  0.90&  0.95& 0.99
\\
        \midrule
            &$\bar{S}$ &  88.6&  88.6&  88.75&  88.59& 
88.77
\\
            &1-$\bar{S}$ &  88.84&  89.16&  88.84&  88.81& 
88.62
\\
            &$\bar{S}$-0.5 &  88.83&  88.46&  88.43&  88.49& 
88.52
\\
            &0.5-$\bar{S}$&  88.78&  88.75&  88.51&  88.67& 
88.63
\\
            &constant&  88.57&  88.67&  89.14&  88.7& 88.76
\\
        \bottomrule
        \end{tabular}
        \subcaption{R@1}
    \end{minipage}    
    \label{tab:scale_sensitivity}
\end{table}
