# Supplementary material for: Object-Aware Query Perturbation for Cross-Modal Image-Text Retrieval
Source: arXiv:2407.12346 source file (2024-09-25)
Supplement: Supplementary file 3 [file eccv_supp_tab3.tex]

\begin{table}
    \centering
\caption{Bold: the best result in each column. Underscore: the best result in each row}
\label{tab:my_label}
    \begin{tabular}{llrrrrrrrcc}
\toprule
 & & Steep& & & & & & Smooth& &\\
          &var&  1 &  6&  12&  24&  48&  96&  192&  & \\
\midrule
 & \multicolumn{8}{c}{Flickr}& &\\
\bottomrule
 org Q-Pert.& & \multicolumn{7}{c}{89.54}& &\\
\hdashline
          &Former&  89.70 &  \second{89.80}&  \first{89.78}&  \first{89.64}&  89.54 &  89.58 &  89.54 
&  & \\
          R@1&Middle&  89.74 &  \first{\second{89.82}}&  89.74 &  89.44 &  89.56 &  89.52 &  89.54 
&  & \\
          &Latter&  \first{\second{89.78}}&  89.66 &  89.64 &  89.42 &  \first{89.74}&  \first{89.60}&  \first{89.60}&  & \\
\bottomrule
 org Q-Pert.& & \multicolumn{7}{c}{88.54}& &\\
\hdashline
          &Former
&  88.70 &  \second{88.96}&  88.80 &  \first{88.80}&  88.70 &  \first{88.64}&  88.52 
&  & \\
          mR@1&Middle
&  \first{88.90}&  \first{\second{88.99}}&  \first{88.97}&  88.45 &  88.60 &  88.50 &  88.50 
&  & \\
          &Latter&  \second{88.73}&  88.59 &  88.44 &  88.22 &  \first{\second{88.73}}&  88.60 &  \first{88.59}&  & \\
\midrule
 & \multicolumn{8}{c}{Flickr-FG}& &\\
\midrule
 org Q-Pert.& & \multicolumn{7}{c}{92.16}& &\\
\hdashline
 & Former
& \first{92.60}& 92.44& \first{92.56}& 92.44& 92.52& \first{\second{92.68}}& \first{92.60}& &\\
 & Middle
& 92.48& \first{92.58}& 92.48& \first{\second{92.72}}& \first{92.68}& 92.48& 92.46
& &\\
 & Latter& 92.42& 92.4& 92.46& 92.54& 92.54& \second{92.66}& 92.52
& &\\
\midrule
 org Q-Pert.& & \multicolumn{7}{c}{91.74}& &\\
\hdashline
 & Former
& \first{92.03}& 91.76& \first{91.81}& 91.72& 91.95& \first{\second{92.10}}& \first{92.03}& &\\
 & 
Middle
& 91.74& \first{91.86}& 91.75& \first{\second{92.14}}& \first{92.10}& 91.93& 91.77
& &\\
 & Latter& 91.73& 91.62& 91.71& 91.80& 91.78& \second{91.93}& 91.84
& &\\
\bottomrule
    \end{tabular}

\end{table}
